# Supplementary material for: Convergence of TD(0) under Polynomial Mixing with Nonlinear Function Approximation
Source: arXiv:2502.05706 source file (2025-05-20)
Supplement: Supplementary file 1 [file 00_related_works.tex]

\subsection*{Table for summary of error bounds for TD(0) algorithm}
\label{app:comparisons}
\begin{table*}[t]
    \centering
    
    \caption{Comparison of error bounds for TD(0) algorithm with linear functional approximation.}
    \setlength{\tabcolsep}{3pt} % Reduce spacing
    \resizebox{\textwidth}{!}{ % Forces table to fit text width
    \begin{tabular}{lccccccc}
        \toprule
        \textbf{Authors} & B. (\citeyear{bhandari18}) & D. (\citeyear{dalal2018finite}) & L. and S.(\citeyear{lakshminarayanan2018linear}) & P. (\citeyear{patil2023finite}) & L.(\citeyear{li2024high}) & S. (\citeyear{samsonov24}) & \textbf{This paper} \\
        \midrule
        \textbf{Algorithm type} & P-R & Last iterate & P-R & P-R & P-R & P-R & Last iterate \\
        \textbf{Step size schedule} & $1/\sqrt{t}$ & $1/k^\kappa$ & constant $\alpha$ & constant $\alpha$ & constant $\alpha$ & constant $\alpha$ & $1/t^\gamma, \gamma>\frac{1}{2}$ \\
        \textbf{Universal step size} & \cmark & \cmark & \cmark & \cmark & \xtimes & \cmark & \cmark \\
        \textbf{Markovian data} & \cmark & \xtimes & \xtimes & \cmark & \xtimes & \cmark & \cmark \\
        \textbf{High-order bounds} & \xtimes & \cmark & \xtimes & \cmark & \cmark & \cmark & \cmark \\
        \textbf{No projection} & \xtimes & \cmark & \cmark & \xtimes & \cmark & \cmark & \cmark\\
        \textbf{Mixing properties} & Geometric & \xtimes & \xtimes & Geometric & \xtimes & Geometric & Polynomial\\
        \textbf{Function} & Linear & Linear & Linear & Linear & Linear & Linear & Deep ReLU Network\\
        \textbf{No Data Dropping} & \cmark & \cmark & \cmark & \cmark & \cmark & \xtimes  & \cmark \\
        \bottomrule
    \end{tabular}
    }
    \vspace{0.5em} % Reduce unnecessary space
    \raggedright
%    \textsuperscript{(1)} (Bhandari et al., 2018) considers constant step size $\alpha = 1/\sqrt{n}$ with $n$ being total number of iterations and provides suboptimal MSE bound of order $\tilde{\mathcal{O}}(1/\sqrt{n})$;
%    \textsuperscript{(2)} (Dalal et al., 2018) uses last iterate and decreasing step size schedule with $\alpha_k = 1/k^\kappa$. Hence, the corresponding bias forgetting rate is sublinear, and the $n$-step MSE is of order $\tilde{\mathcal{O}}(1/n^\kappa)$;
%    \textsuperscript{(3)} (Patil et al., 2023) uses projections to prove the concentration bounds, and the definition of the projection set involves the unknown parameter $\theta_*$. 
\end{table*}
